# Supplementary material for: Ensnarled: On the topological linkage of spatially embedded network pairs
Source: arXiv:2208.11662 source file (2023-08-05)
Supplement: Supplementary file 1 [file figure_6.tex]

\begin{figure}[h]
\centering
\includegraphics[scale=.5]{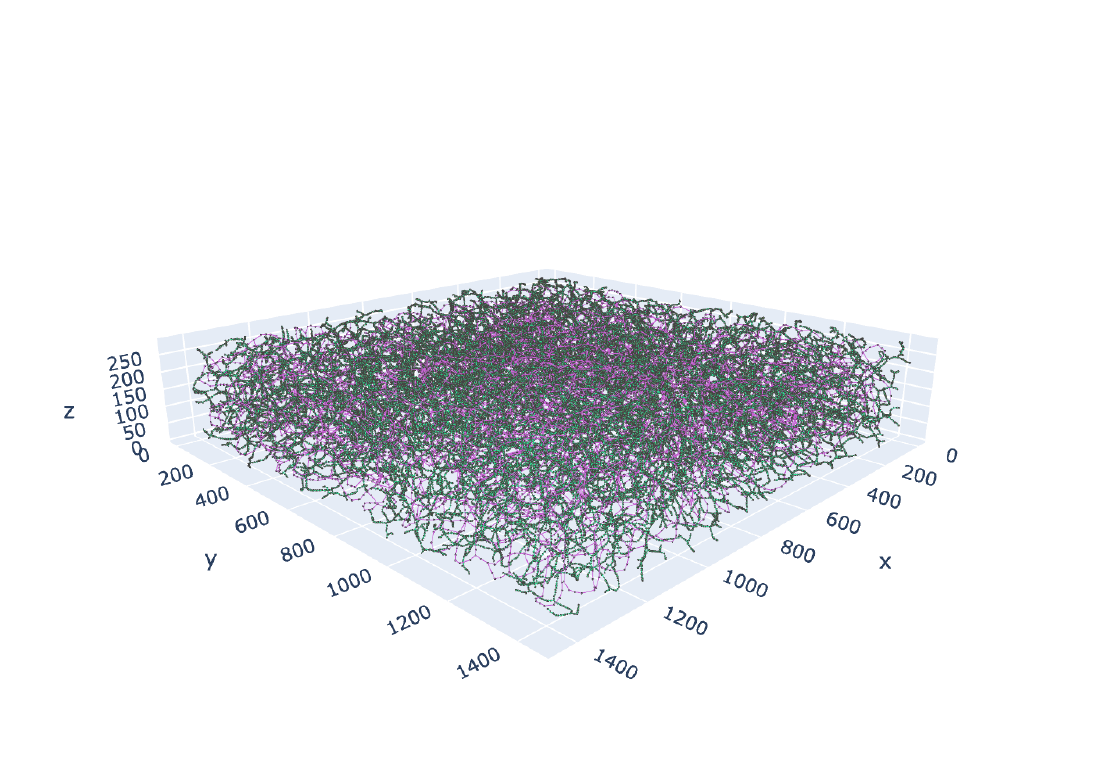}
	\caption{
	Network skeletons of vasculature in liver tissue:
%	\subR{fig:classificationLiver}
Sinusoids (magenta) and bile canaliculi (green) segment in the liver acinus.
	}\label{fig:classificationLiver}
\end{figure}
