# Supplementary material for: Ensnarled: On the topological linkage of spatially embedded network pairs
Source: arXiv:2208.11662 source file (2023-08-05)
Supplement: Supplementary file 2 [file figure_7.tex]

\begin{figure}[h]
\centering
\subfloat[$\chi \in [0,150)$]{
\label{fig:classificationLiver0}
\hspace{-.8cm}
	\includegraphics[scale=.275]{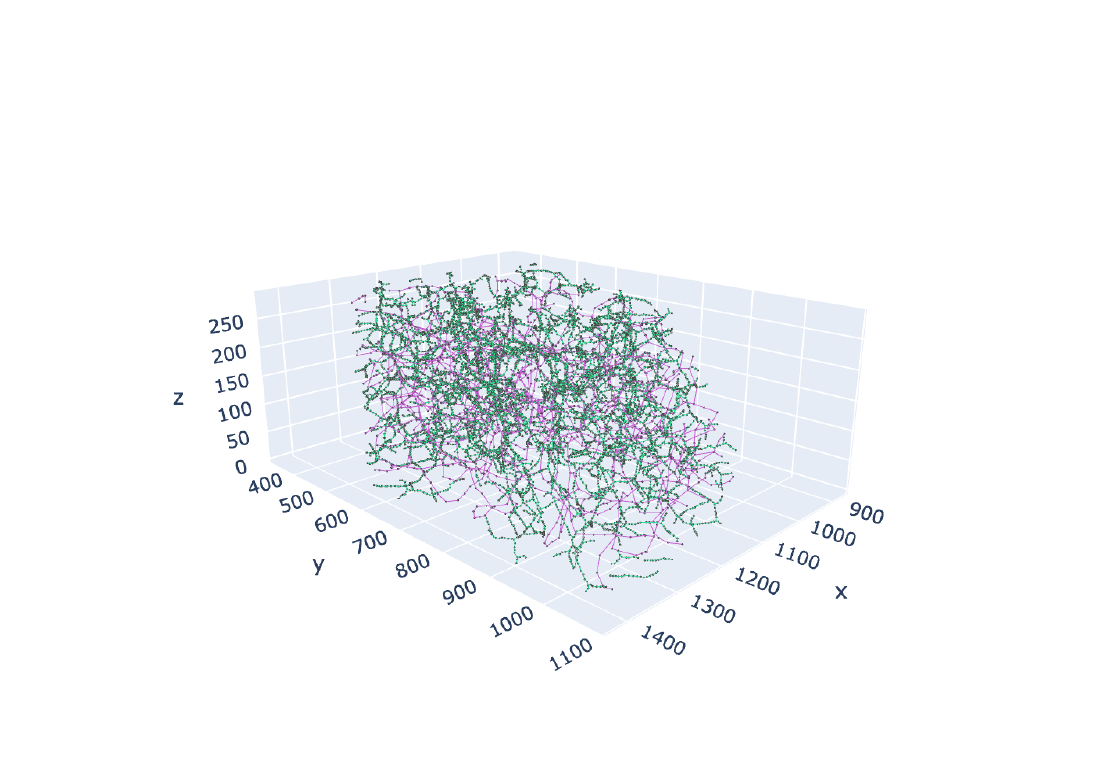}
	}
	\subfloat[$\chi \in [150,300)$]{
	\hspace{-1.1cm}
	\includegraphics[scale=.275]{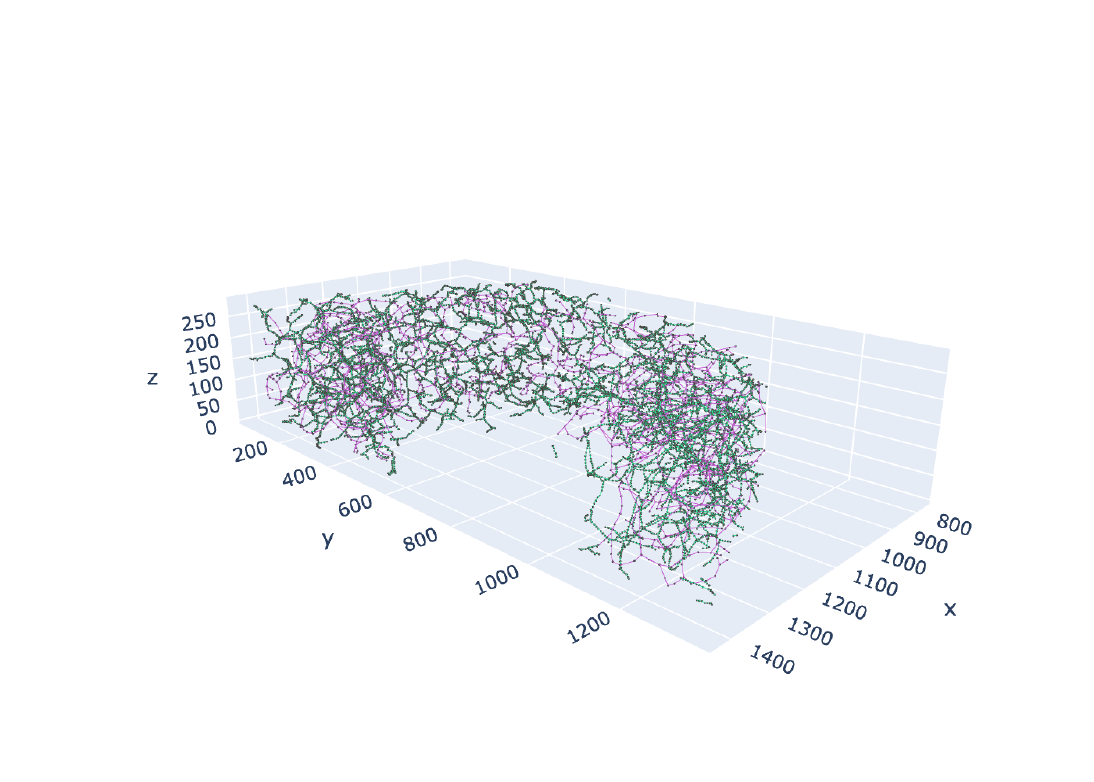}
	}\\
	\subfloat[$\chi \in [300,450)$]{
	\hspace{-.8cm}
	\includegraphics[scale=.275]{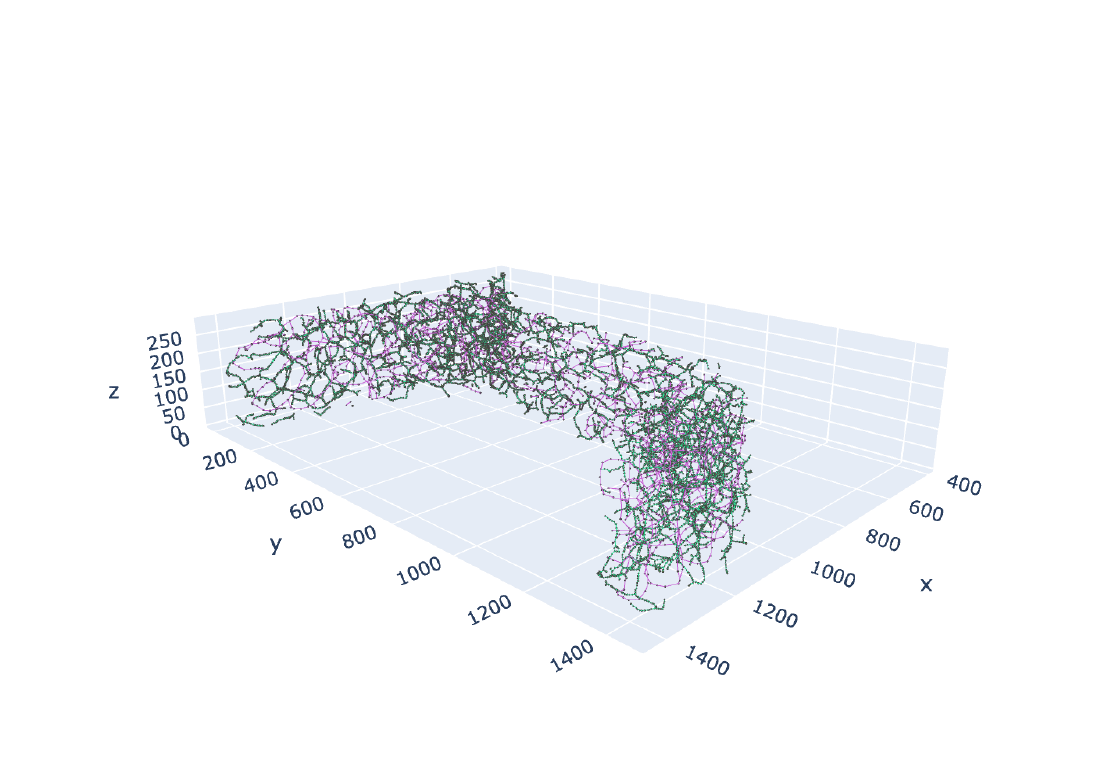}
	}
	\subfloat[$\chi \in [450,600)$]{
	\hspace{-1.1cm}
	\includegraphics[scale=.275]{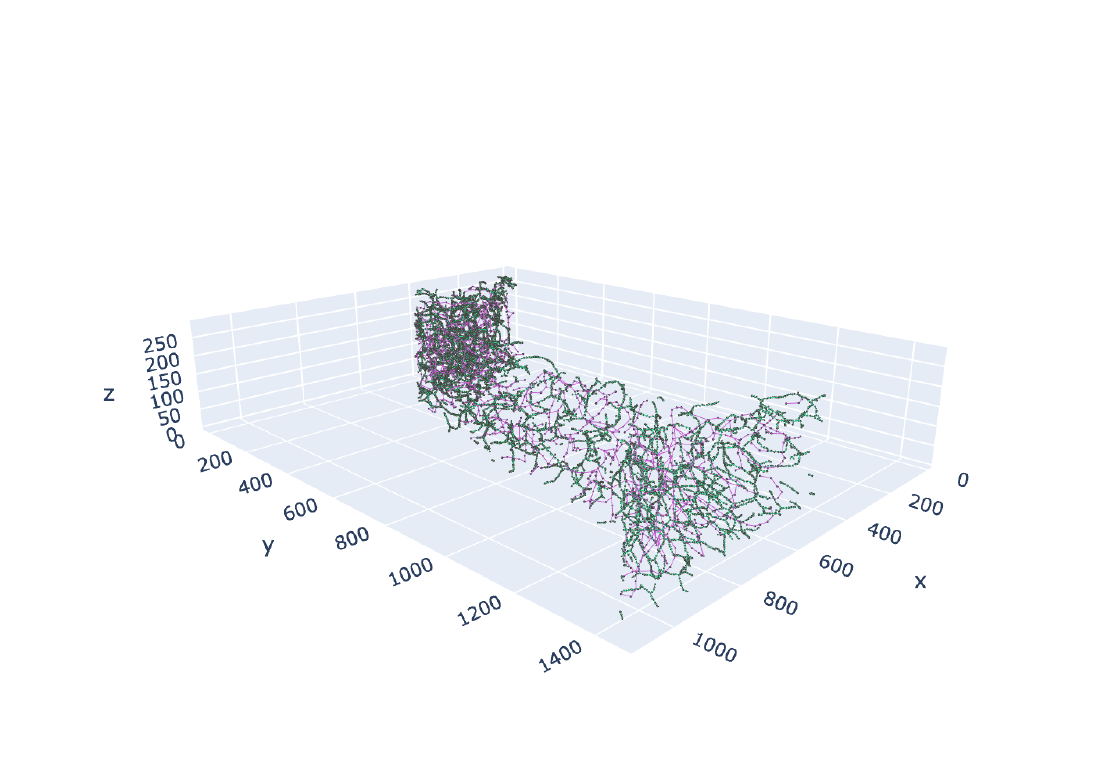}
	}\\
	\subfloat[$\chi \in [600,750)$]{
	\hspace{-.8cm}
	\includegraphics[scale=.275]{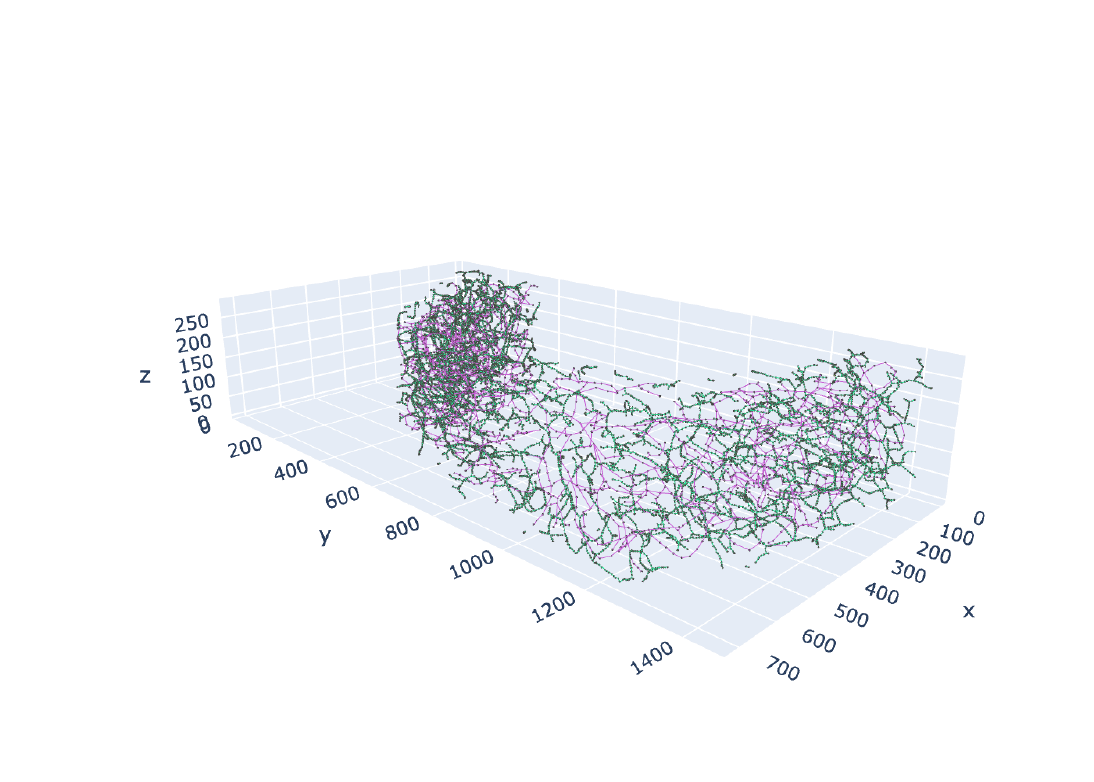}
	}
	\subfloat[$\chi \in [750,900)$]{
	\label{fig:classificationLiver1}
	\hspace{-1.1cm}
	\includegraphics[scale=.275]{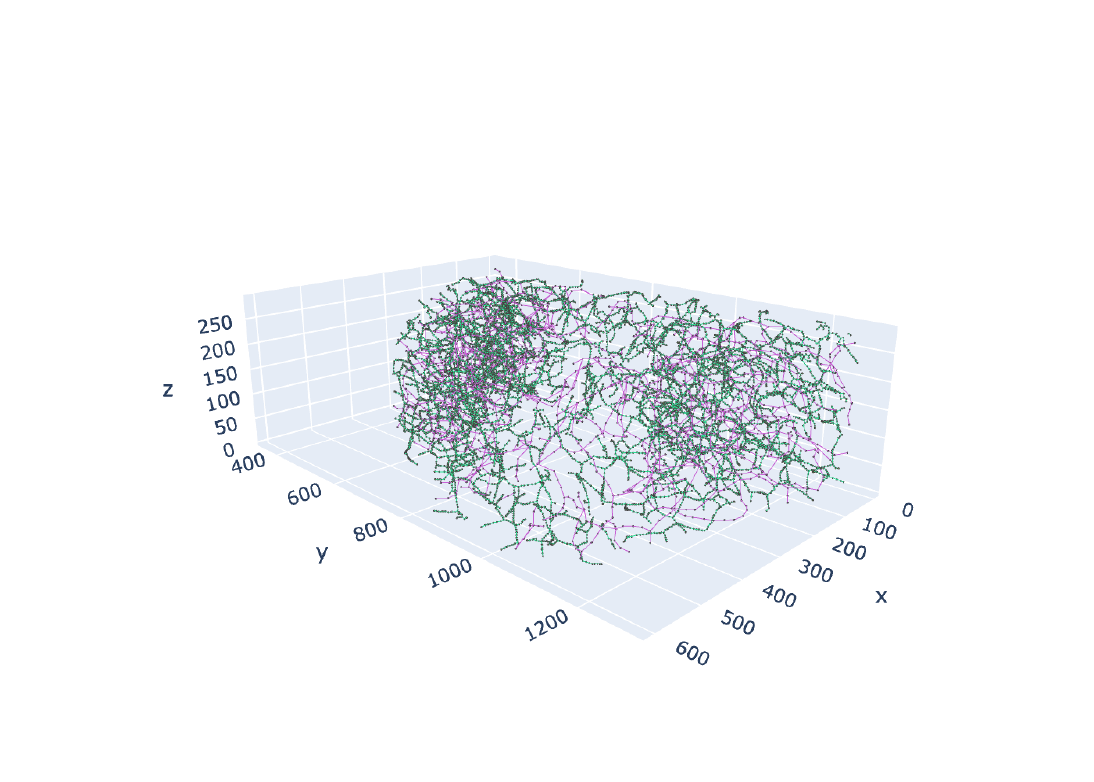}
	}
	\caption{
	Network skeletons of vasculature in liver tissue:
 Separation the liver acinus vasculature mesh into regular $\Delta\chi=150$ sections for further analysis of the zonated linkage behavior.
	}\label{fig:classificationLiverZonation}
\end{figure}
