# Supplementary material for: Ensnarled: On the topological linkage of spatially embedded network pairs
Source: arXiv:2208.11662 source file (2023-08-05)
Supplement: Supplementary file 4 [file figure_9.tex]

\begin{figure}[h]
\centering
\subfloat[]{
	\includegraphics[scale=1.]{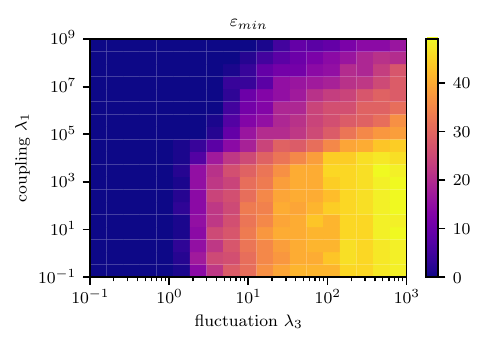}
	}\\
	\subfloat[]{
	\includegraphics[scale=1.]{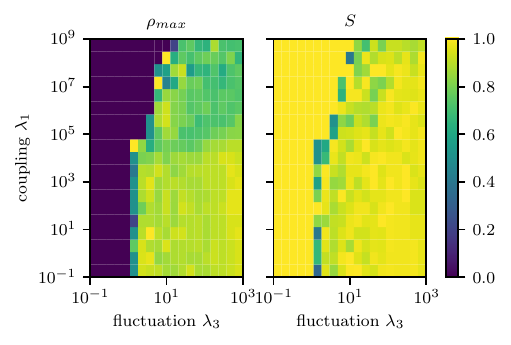}
	}
	\caption{
	Classification of entangled, adapting and repulsively coupled systems ($\nu > 1$)
	}\label{fig:classificationAdaptiveRep}
\end{figure} 

\begin{figure}[h]
\centering
\subfloat[]{
	\includegraphics[scale=1.]{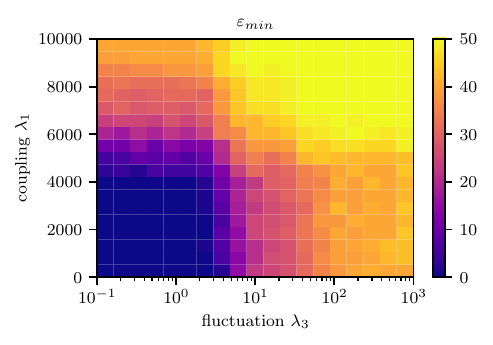}
	}\\
	\subfloat[]{
	\includegraphics[scale=1.]{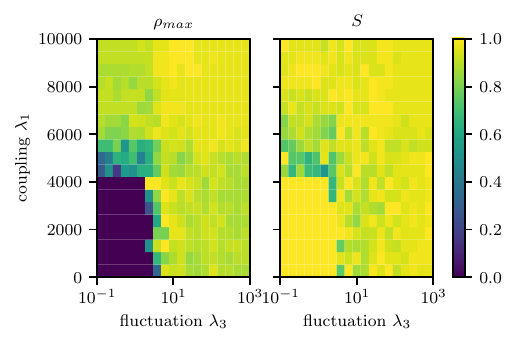}
	}
	\caption{
	Classification of entangled, adapting and attractively coupled systems ($\nu < -1$) systems. 
	}\label{fig:classificationAdaptiveAtt}
\end{figure}
